# Supplementary material for: Understanding Data Movement in Tightly Coupled Heterogeneous Systems: A Case Study with the Grace Hopper Superchip
Source: arXiv:2408.11556 source file (2024-08-26)
Supplement: Supplementary file 1 [file appendix.tex]

\section{Appendix}
\begin{figure}[h]
\centering
\includegraphics[width=\linewidth]{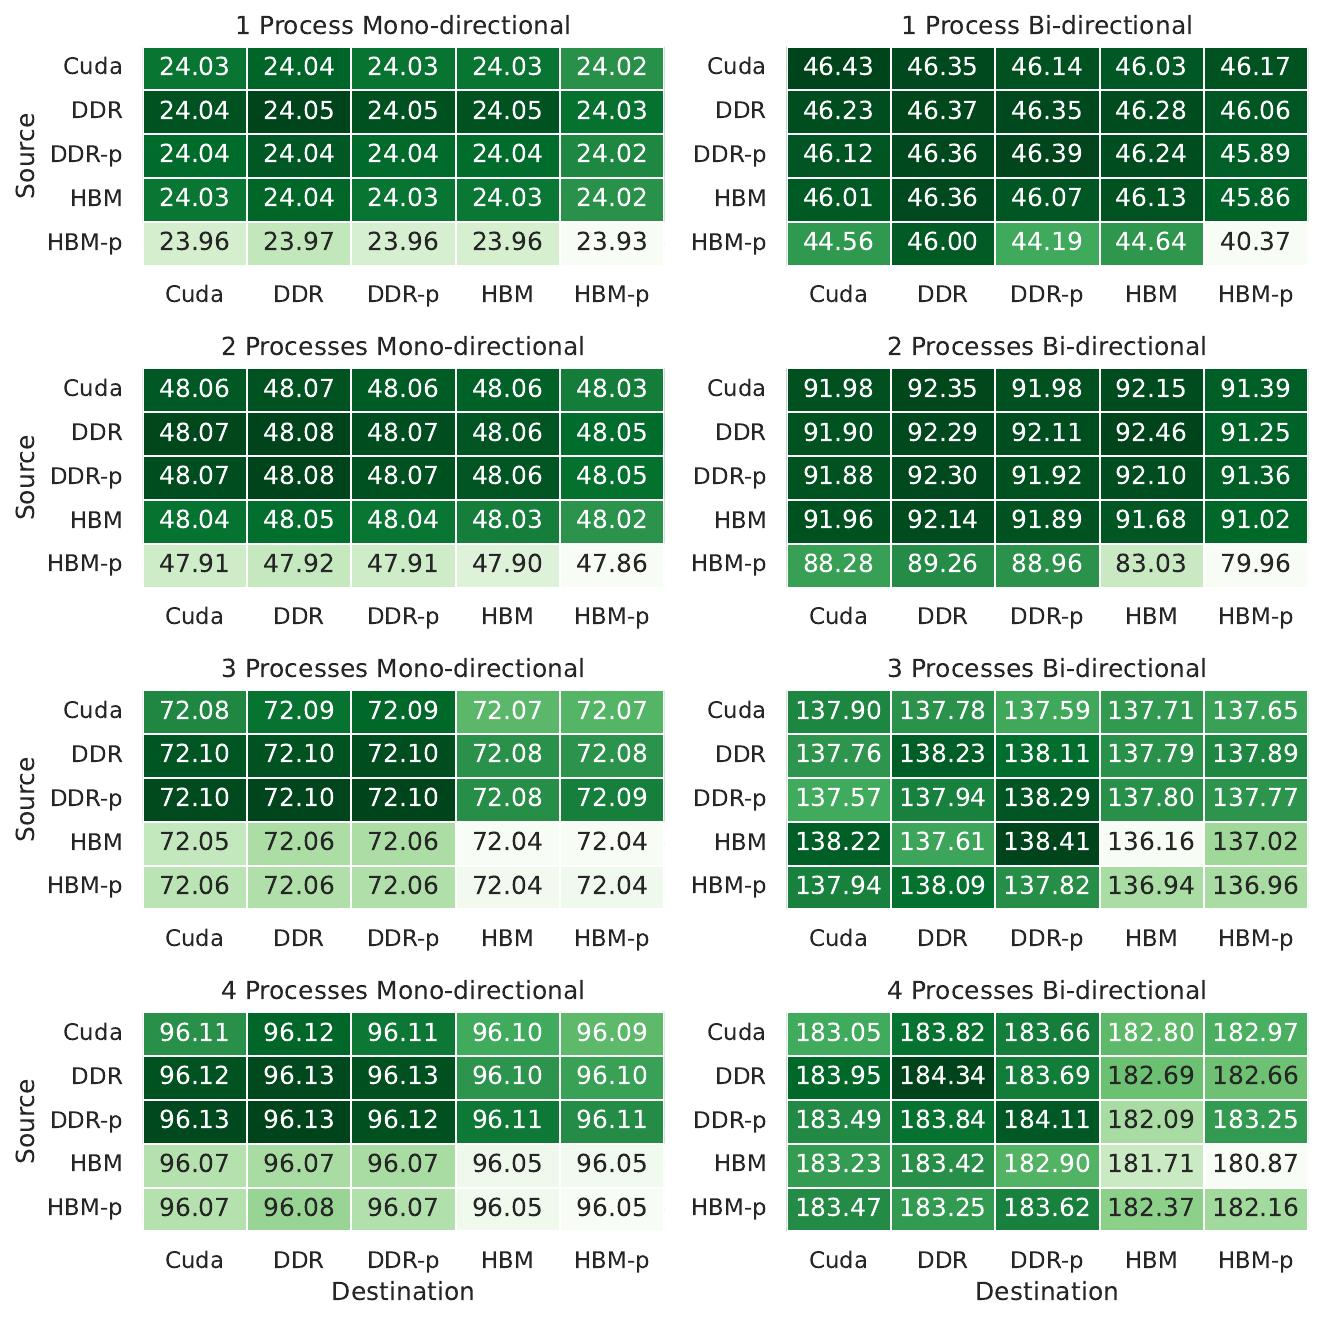}
\caption{Throughput of memory transfers using \texttt{MPI\_Isend} and \texttt{MPI\_Irecv} in GB/s of a 4GB buffer. Source and destination buffers change in placement. Remote and local memories are from the perspective of the GPU allocated to the process.}
\label{mpi_send_recv}
\end{figure}

\subsubsection{STREAM}
\begin{figure}[h]
\centering
\includegraphics[width=0.3\textwidth]{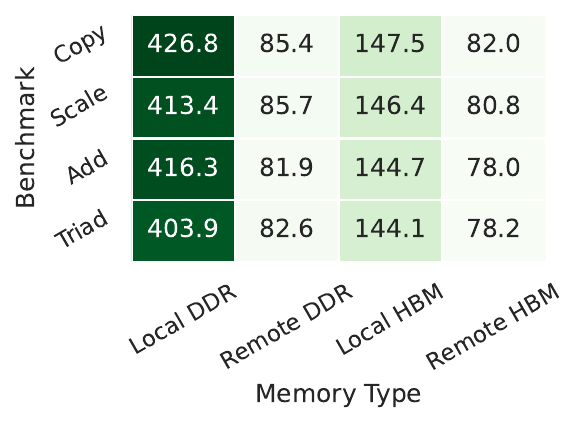}
\end{figure}
STREAM is a popular synthetic benchmark program which is commonly used to measure sustained throughput of vector kernels. GPU-STREAM is a STREAM inspired benchmark that targets GPUs. We modify GPU-STREAM in order to add support for allocating memory in different ways. Both STREAM and GPU-STREAM are run with default measurement settings, and with float arrays of 2\^30 elements.
All STREAM kernels are memory bound. Copy and Scale read from one array and write to one array, while Add and Triad read from two arrays and write to one array. Throughput is calculated as (\#N read bytes + \#N written bytes) / time, making different kernels comparable.
